# Supplementary material for: Union: A Unified HW-SW Co-Design Ecosystem in MLIR for Evaluating Tensor Operations on Spatial Accelerators
Source: arXiv:2109.07419 source file (2021-11-07)
Supplement: Supplementary file 1 [file appendix.tex]

\appendix
We explain how to reproduce the results using the artifacts that we provide.
\subsection{Get ready for Union}
We provide a docker image which includes all the necessary dependencies and source codes. We also built the binary files for convenience, but you can also build by yourself if you want. 
Please refer to the detailed instructions at the GitHub repository\footnote{\url{https://github.com/union-codesign/union-pact21ae}} for how to build.
In the paper, we provide three case studies with various workloads (Figure 8, 10, 11). 
There are scripts for running each of them.
We also provide an excel file (\textit{opt\_results\_reproduce.xlsx}) which summarizes all the results.
For your reference, we also include time taken for each experiment (this might be different depending on your machine, but we believe this can give you some estimation).
We used Intel(R) Xeon(R) Silver 4210 CPU @ 2.20GHz with 32GB memory. 
Since we also included build files in the image, the size of image is very large (mainly due to the LLVM build).
In this document, we assume that you installed docker in your machine.
To start with Union, get the docker image and run a container using the image.
%https://docs.docker.com/engine/install/ubuntu/
\begin{lstlisting}[language=bash]
  $ sudo docker pull uniondevelopergroup/union
  $ sudo docker run --name union-check -d -i -t uniondevelopergroup/union
  $ docker attach union-check
\end{lstlisting}

%1. If you do not have docker in your machine, please follow the instructions in the following website.

%2. Once you install your docker, you can get the docker image for UNION from the docker hub. 

%3. Now you can run the docker image.

%4. Next, you can get into the docker container which includes all the source codes and binaries.

\subsection{\union-frontend}
Union-frontend lowers the code written in high level language into dialects that we are targeting. We also implemented several passes to check whether the operation is conformable to certain cost models. We implemented simple tests so that you can check whether they work as expected. You can run the commands below to check. For more details, please take a look at README.md.

\begin{lstlisting}[language=bash]
  $ cd /home/union-pact21ae/union-frontend
  $ ninja check
\end{lstlisting}

\subsection{\union-opt}
Union-opt runs the target cost model to find the optimal mapping and return stats. 
In the \textit{/home/union-pact21ae/union-opt/exp} directory, scripts are available to reproduce the numbers used in the paper (and \textit{/home/union-pact21ae/union-opt/exp/opt\_results\_reproduce.xlsx}). 
After running a \textit{run\_case\_study\_n.sh} script, the result will be saved in the result folder. 
At the end of each file, you can find the optimal EDP and you can match that number with the one in the excel file. 
Since running the entire \textit{run\_case\_study\_n.sh} might take long, you can also run individual experiments as well. 
Please take a look at \textit{run\_case\_study\_n.sh} scripts, and run the specific experiment you want to reproduce.
For case-study 1, we used intensli2, ccsd7, and ccsdt4.
For case-study 2 and 3, we used resnet\_1-3, dlrm\_1-3, and bert\_1-3. 
You can run each experiment using the following for the case study 1 or 2 (with the target workload and number).

\begin{lstlisting}[language=bash]
$ cd /home/union-pact21ae/union-opt/exp/{workload}
$ ./run_case_study_{number}.sh
\end{lstlisting}

For example, you can run the case study 1 with intensli2 using the followings.

\begin{lstlisting}[language=bash]
$ cd /home/union-pact21ae/union-opt/exp/intensli2
$ ./run_case_study_1.sh
\end{lstlisting}

For the case study 3, you can run the followings.

\begin{lstlisting}[language=bash]
$ cd /home/union-pact21ae/union-opt/exp/{workload}/case-study-3
$ ./run_case_study_3.sh
\end{lstlisting}

For example, you can run the case study 3 with resnet\_1 using the followings.

\begin{lstlisting}[language=bash]
$ cd /home/union-pact21ae/union-opt/exp/resnet_1/case-study-3
$ ./run_case_study_3.sh
\end{lstlisting}
